# Supplementary material for: QDGset: A Large Scale Grasping Dataset Generated with Quality-Diversity
Source: arXiv:2410.02319 source file (2024-10-03)
Supplement: Supplementary file 1 [file appendices.tex]

%%%%%%%%%%%%%%%%%%%%%%%%%%%%%%%%%%%%%%%%%%%%%%%%%%%%%%%%%%%%%%%%%%%%%%%
%                       Supplementary materials
%%%%%%%%%%%%%%%%%%%%%%%%%%%%%%%%%%%%%%%%%%%%%%%%%%%%%%%%%%%%%%%%%%%%%%%

\clearpage
\appendices

\begin{table*}[t]
\centering
\begin{tabular}{ || c || c | c | c | c | c | c ||}

\hline

\makecell{\textbf{Objects source}} & \makecell{\textbf{Num.}\\\textbf{objects}}  & \makecell{\textbf{Num.}\\\textbf{grasps}} & \makecell{\textbf{Mean grasps}\\\textbf{per object}}  & \makecell{\textbf{Std grasps}\\\textbf{per object}} & \makecell{\textbf{Num.}\\\textbf{no success}} & \makecell{\textbf{Objects type}} \\

\hhline{||=||=|=|=|=|=|=||}

3DNet & 1\,175 & 4\,449\,168 & 3\,787 & 1\,621 & 0 & Daily (intermediate complexity: dishes, shoes, tools, keyboards, toys ...)  \\
\hline
KIT & 129 & 437\,380 & 3\,391  & 344 & 0 & Daily (simple: cylinders, boxes + some more complex objects)  \\
\hline
YCB & 94 & 145\,626 & 1\,549  & 1\,146 & 12 & Daily (intermediate complexity: dishes, tools, toys)  \\
\hline
Graspnet1Billion & 87 & 179\,887 & 2\,044 & 894 & 2 & Daily (intermediate complexity: dishes, tools, toys)  \\
\hline
ShapeNet & 25\,837 & 33\,214\,669 & 1\,286 & 1\,392 & 8\,691 & Human-scaled (high complexity: street and home furnitures, plumbing, vehicules, music instruments, ...) \\
\hline
EGAD & 2\,330 & 4\,604\,776 & 1\,977 & 395 & 0 & Adversarial  \\

\hhline{||=||=|=|=|=|=|=||}

3DNet\textit{-aug} & 9\,706 & 17\,018\,746 & 1\,753 & 1\,045 & 69 & Daily  \\
\hline
KIT\textit{-aug} & 1290 & 1\,527\,167 & 1\,535 & 359 & 0 & Daily  \\

\hhline{||=||=|=|=|=|=|=||}

\makecell{\textbf{Dataset}} & \makecell{\textbf{Num.}\\\textbf{objects}}  & \makecell{\textbf{Num.}\\\textbf{grasps}} & \makecell{\textbf{Mean grasps}\\\textbf{per object}} & \makecell{\textbf{Std grasps}\\\textbf{per object}} & \makecell{\textbf{Num.}\\\textbf{failures}} & \makecell{\textbf{Objects type}} \\

\hline

QDGSet\textit{-core} & 29\,652 & 43\,031\,506 & 1\,451 & 1\,446 & 8\,705 & Daily, human-scaled, adversarial  \\
\hline
QDGSet & 40\,648 & 61\,577\,419 & 1\,526 & 1\,348 & 8\,774 & Daily, human-scaled, adversarial  \\

\hline

\end{tabular}
\caption{\textbf{QDG-Set description.} Object sources with *-aug in their name corresponds to augmented object datasets. QDGSet\textit{-core} contains no augmented objects. QDGSet contains all the generated grasps on any kind of objects.}
\label{table:dataset_comparison_detailed}
\end{table*}

\begin{figure}[t]
  \centering
\centering
  \includegraphics[width=\columnwidth]{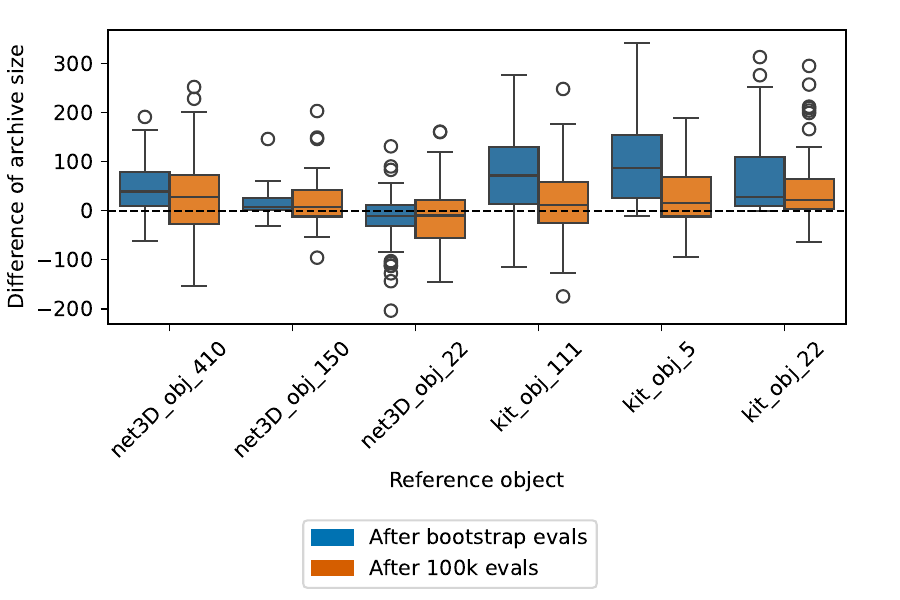}
  \caption{\textbf{Sample efficiency evaluation: details.} Difference of number of generated grasps when stopping at bootstrap time, or on the long run.}
  \label{fig:appendix_boxplot_sample_efficiency_detailed}
\end{figure}
